# Supplementary material for: A strange relationship between 2d CFT and 4d gauge theory
Source: arXiv:1108.5632 ancillary file (2011-08-29)
Supplement: Supplementary file 1 [file comparison-su2.pdf]

---

## Comparison of the norm of the coherent state of Virasoro algebra and the instanton partition function of SU(2).

---

### CFT

- **B** Evaluates  $\langle 0 | LLL \dots LLLL | 0 \rangle$  by commutation relations.

```
In[1]:= B[{ } ] := 1
In[2]:= B[{n_, x___}] /; n < 0 := 0
In[3]:= B[{n_, x___}] /; n == 0 := Δ B[{x}]
In[4]:= B[{x___, n_}] /; n > 0 := 0
In[5]:= B[{x___, n_}] /; n == 0 := Δ B[{x}]
In[6]:= B[{l___, m_, n_, r___}] /; (m ≠ -n && m ≥ 0 && n < 0) :=
  (m - n) B[{l, m + n, r}] + B[{l, n, m, r}]
In[7]:= B[{l___, m_, n_, r___}] /; (m == -n && m ≥ 0 && n < 0) :=
  (m - n) B[{l, m + n, r}] + B[{l, n, m, r}] + c m (m^2 - 1) / 12 B[{l, r}]
```

- **Kac matrix.**

```
In[8]:= Kac[n_] := Kac[n] = Module[{par = IntegerPartitions[n]},
  Table[B[Join[Reverse[par[[i]]], -par[[j]]], {i, 1, Length[par]}, {j, 1, Length[par]}]]
In[9]:= IKac[n_] := Inverse[Kac[n]]
```

- $\langle w | w \rangle$  as the entry  $Kac^{(-1)}[\{1^n\}, \{1^n\}]$ . Uses the fact  $\{1^n\}$  appears last in `Partitions[n]`. `ww[i]` is the contribution from *i*-th descendants.

```
In[10]:= ww[n_] := Module[{par = IntegerPartitions[n]}, IKac[n][[Length[par], Length[par]]] λλ^n
```

---

## Regularized Volume = Nekrasov parittion function

```
In[11]:= DualPartition[l_] := Module[{i}, Table[Length[Select[l, (# >= i) &]], {i, 1, l[[1]]}]]
In[12]:= DualPartition[{ } ] = { };
In[13]:= get[Y_, i_] := If[i > Length[Y], 0, Y[[i]]]
In[14]:= arm[Y_, {i_, j_}] := get[Y, i] - j
In[15]:= leg[Y_, {i_, j_}] := get[DualPartition[Y], j] - i
In[16]:= boxes[Y_] := Join@@Module[{i, j}, Table[Table[{i, j}, {j, 1, Y[[i]]}], {i, 1, Length[Y]}]]
In[17]:= e[a_, Y1_, Y2_, s_] := a - ε1 leg[Y2, s] + ε2 (arm[Y1, s] + 1)
```

- **Contribution of a W-boson**

```
In[18]:= fromWa[a_, bb_, Y1_, Y2_] :=
  (Times @@ (e[a - bb, Y1, Y2, #] (ε1 + ε2 - e[a - bb, Y1, Y2, #])) & /@ boxes[Y1])
```

- **Contribution of a U(2) vector multiplet**

```
In[19]:= fromSU2V[a_, Y1_, Y2_] :=
  1 / (fromWa[a, a, Y1, Y1] fromWa[a, -a, Y1, Y2] fromWa[-a, a, Y2, Y1] fromWa[-a, -a, Y2, Y2])
```

```
In[20]:= youngPairs[k_] := youngPairs[k] = Join @@ Module[{i},
  Join @@ Table[Outer[List, IntegerPartitions[i], IntegerPartitions[k - i], 1], {i, 0, k}]]
```

■ i-instanton contribution

```
In[21]:= pure[i_] := (Plus @@ (fromSU2V[a, #[[1]], #[[2]]] & /@ youngPairs[i])) q^(i)
```

## Comparison

```
In[22]:= Q2 := (ε1 + ε2) ^ 2 / (ε1 ε2);
```

```
In[23]:= dic = {Δ → Q2 / 4 - a^2 / (ε1 ε2), c → 1 + 6 Q2, λλ → q / (ε1 ε2) ^ 2}
```

```
Out[23]= {Δ → - $\frac{a^2}{\epsilon_1 \epsilon_2} + \frac{(\epsilon_1 + \epsilon_2)^2}{4 \epsilon_1 \epsilon_2}$ , c →  $1 + \frac{6 (\epsilon_1 + \epsilon_2)^2}{\epsilon_1 \epsilon_2}$ , λλ →  $\frac{q}{\epsilon_1^2 \epsilon_2^2}$ }
```

```
In[24]:= k = 1;
```

```
In[25]:= gauge = pure[k]
```

```
Out[25]= q  $\left( \frac{1}{2 a \epsilon_1 \epsilon_2 (-2 a + \epsilon_1 + \epsilon_2)} - \frac{1}{2 a \epsilon_1 \epsilon_2 (2 a + \epsilon_1 + \epsilon_2)} \right)$ 
```

```
In[26]:= cft = ww[k]
```

```
Out[26]=  $\frac{\lambda \lambda}{2 \Delta}$ 
```

```
In[27]:= gauge - (cft /. dic) // FullSimplify
```

```
Out[27]= 0
```

```
In[28]:= k = 2;
```

```
In[29]:= gauge = pure[k]
```

```
Out[29]= q^2  $\left( \frac{1}{\epsilon_1^2 (-2 a + \epsilon_1) (2 a + \epsilon_1) \epsilon_2^2 (-2 a + \epsilon_2) (2 a + \epsilon_2)} + \right.$   

 $\frac{1}{4 a (2 a - \epsilon_1) \epsilon_1^2 \epsilon_2 (-\epsilon_1 + \epsilon_2) (-2 a + \epsilon_1 + \epsilon_2) (-2 a + 2 \epsilon_1 + \epsilon_2)}$  -  

 $\frac{1}{4 a (-2 a - \epsilon_1) \epsilon_1^2 \epsilon_2 (-\epsilon_1 + \epsilon_2) (2 a + \epsilon_1 + \epsilon_2) (2 a + 2 \epsilon_1 + \epsilon_2)}$  +  

 $\frac{1}{4 a \epsilon_1 (2 a - \epsilon_2) (\epsilon_1 - \epsilon_2) \epsilon_2^2 (-2 a + \epsilon_1 + \epsilon_2) (-2 a + \epsilon_1 + 2 \epsilon_2)}$  -  

 $\left. \frac{1}{4 a \epsilon_1 (-2 a - \epsilon_2) (\epsilon_1 - \epsilon_2) \epsilon_2^2 (2 a + \epsilon_1 + \epsilon_2) (2 a + \epsilon_1 + 2 \epsilon_2)} \right)$ 
```

```
In[30]:= Kac[k] // MatrixForm // Simplify
```

```
Out[30]//MatrixForm=
```

```
 $\begin{pmatrix} \frac{1}{2} (c + 8 \Delta) & 6 \Delta \\ 6 \Delta & 4 \Delta (1 + 2 \Delta) \end{pmatrix}$ 
```

```
In[31]:= cft = ww[k]
```

```
Out[31]=  $\frac{\left( \frac{c}{2} + 4 \Delta \right) \lambda \lambda^2}{2 c \Delta - 20 \Delta^2 + 4 c \Delta^2 + 32 \Delta^3}$ 
```

In[32]:= **gauge - (cft /. dic) // FullSimplify**

Out[32]= 0

In[33]:= **k = 3;**

In[34]:= **gauge = pure[k]**

$$\text{Out[34]} = q^3 \left( \frac{1}{4 a \epsilon_1^3 (2 a + \epsilon_1) (-2 a + 2 \epsilon_1) \epsilon_2^2 (-2 a + \epsilon_2) (-\epsilon_1 + \epsilon_2) (2 a - \epsilon_1 + \epsilon_2) (-2 a + \epsilon_1 + \epsilon_2)} - \right. \\ \frac{1}{4 a \epsilon_1^3 (-2 a + \epsilon_1) (2 a + 2 \epsilon_1) \epsilon_2^2 (2 a + \epsilon_2) (-\epsilon_1 + \epsilon_2) (-2 a - \epsilon_1 + \epsilon_2) (2 a + \epsilon_1 + \epsilon_2)} + \\ \frac{1}{12 a (2 a - 2 \epsilon_1) (2 a - \epsilon_1) \epsilon_1^3 \epsilon_2 (-2 \epsilon_1 + \epsilon_2) (-\epsilon_1 + \epsilon_2) (-2 a + \epsilon_1 + \epsilon_2) (-2 a + 2 \epsilon_1 + \epsilon_2) (-2 a + 3 \epsilon_1 + \epsilon_2)} - \frac{1}{12 a (-2 a - 2 \epsilon_1) (-2 a - \epsilon_1) \epsilon_1^3 \epsilon_2 (-2 \epsilon_1 + \epsilon_2) (-\epsilon_1 + \epsilon_2) (2 a + \epsilon_1 + \epsilon_2) (2 a + 2 \epsilon_1 + \epsilon_2) (2 a + 3 \epsilon_1 + \epsilon_2)} \Big) + \\ \frac{1}{4 a \epsilon_1^2 (-2 a + \epsilon_1) (\epsilon_1 - \epsilon_2) (2 a + \epsilon_1 - \epsilon_2) \epsilon_2^3 (2 a + \epsilon_2) (-2 a + \epsilon_1 + \epsilon_2) (-2 a + 2 \epsilon_2)} - \\ \frac{1}{4 a \epsilon_1^2 (2 a + \epsilon_1) (\epsilon_1 - \epsilon_2) (-2 a + \epsilon_1 - \epsilon_2) \epsilon_2^3 (-2 a + \epsilon_2) (2 a + \epsilon_1 + \epsilon_2) (2 a + 2 \epsilon_2)} + \\ \frac{1}{2 a (2 a - \epsilon_1) \epsilon_1^2 (2 a - \epsilon_2) (2 \epsilon_1 - \epsilon_2) \epsilon_2^2 (-2 a + \epsilon_1 + \epsilon_2) (-2 a + 2 \epsilon_1 + \epsilon_2) (-\epsilon_1 + 2 \epsilon_2) (-2 a + \epsilon_1 + 2 \epsilon_2)} - \frac{1}{2 a (-2 a - \epsilon_1) \epsilon_1^2 (-2 a - \epsilon_2) (2 \epsilon_1 - \epsilon_2) \epsilon_2^2 (2 a + \epsilon_1 + \epsilon_2) (2 a + 2 \epsilon_1 + \epsilon_2) (-\epsilon_1 + 2 \epsilon_2) (2 a + \epsilon_1 + 2 \epsilon_2)} \Big) + \\ \frac{1}{12 a \epsilon_1 (2 a - 2 \epsilon_2) (\epsilon_1 - 2 \epsilon_2) (2 a - \epsilon_2) (\epsilon_1 - \epsilon_2) \epsilon_2^3 (-2 a + \epsilon_1 + \epsilon_2) (-2 a + \epsilon_1 + 2 \epsilon_2) (-2 a + \epsilon_1 + 3 \epsilon_2)} - \frac{1}{12 a \epsilon_1 (-2 a - 2 \epsilon_2) (\epsilon_1 - 2 \epsilon_2) (-2 a - \epsilon_2) (\epsilon_1 - \epsilon_2) \epsilon_2^3 (2 a + \epsilon_1 + \epsilon_2) (2 a + \epsilon_1 + 2 \epsilon_2) (2 a + \epsilon_1 + 3 \epsilon_2)} \Big)$$

In[35]:= **Kac[k] // MatrixForm // Simplify**

Out[35]//MatrixForm=

$$\begin{pmatrix} 2 (c + 3 \Delta) & 10 \Delta & 24 \Delta \\ 10 \Delta & \Delta (8 + c + 8 \Delta) & 12 \Delta (1 + 3 \Delta) \\ 24 \Delta & 12 \Delta (1 + 3 \Delta) & 24 \Delta (1 + 3 \Delta + 2 \Delta^2) \end{pmatrix}$$

In[36]:= **cft = ww[k]**

$$\text{Out[36]} = \left( (16 c \Delta + 2 c^2 \Delta - 52 \Delta^2 + 22 c \Delta^2 + 48 \Delta^3) \lambda \lambda^3 \right) / (96 c \Delta^2 + 48 c^2 \Delta^2 - 960 \Delta^3 - 624 c \Delta^3 + 144 c^2 \Delta^3 + 4896 \Delta^4 - 240 c \Delta^4 + 96 c^2 \Delta^4 - 6816 \Delta^5 + 1056 c \Delta^5 + 2304 \Delta^6)$$

In[37]:= **gauge - (cft /. dic) // FullSimplify**

Out[37]= 0
