# Supplementary material for: A strange relationship between 2d CFT and 4d gauge theory
Source: arXiv:1108.5632 ancillary file (2011-08-29)
Supplement: Supplementary file 2 [file comparison-su3.pdf]

---

## Comparison of the norm of the coherent state of $W_3$ algebra and the instanton partition function of SU(3). See Taki-kun's paper 0912.4789 for basics.

---

### Instanton.

- dual (or transposed) partition.

```
In[1]:= DualPartition[l_] := Module[{i}, Table[Length[Select[l, (# >= i) &]], {i, 1, 1[[1]]}]]
In[2]:= DualPartition[{}] = {};
In[3]:= get[Y_, i_] := If[i > Length[Y], 0, Y[[i]]]
In[4]:= YoungTuples[1, tot_] := {#} & /@ IntegerPartitions[tot]
In[5]:= YoungTuples[n_, tot_] :=
  YoungTuples[n, tot] = Flatten[Table[Flatten[Outer[Prepend[#2, #1] &,
    IntegerPartitions[r], YoungTuples[n - 1, tot - r], 1, 1], 1], {r, 0, tot}], 1]
```

- arm and leg lengths

```
In[6]:= arm[Y_, {i_, j_}] := get[Y, i] - j
In[7]:= leg[Y_, {i_, j_}] := get[DualPartition[Y], j] - i
In[8]:= boxes[Y_] := Join@@Module[{i, j}, Table[Table[{i, j}, {j, 1, Y[[i]]}], {i, 1, Length[Y]}]]
In[9]:= e[a_, Y1_, Y2_, s_] := a -  $\epsilon_1$  leg[Y2, s] +  $\epsilon_2$  (arm[Y1, s] + 1)
```

- Contribution of a W-boson

```
In[10]:= fromWone[a_, b_, Y1_, Y2_] :=
  (Times @@ (e[a - b, Y1, Y2, #] (e1 + e2 - e[a - b, Y1, Y2, #])) & /@ boxes[Y1]))
In[11]:= SUNdenom[as_, ys_] := Module[{n = Length[as], i, j},
  Product[fromWone[as[[i]], as[[j]], ys[[i]], ys[[j]], {i, 1, n}, {j, 1, n}]]
In[12]:= pure[i_] := (Plus @@ (1 / SUNdenom[{a1, a2, -a1 - a2}, #] & /@ YoungTuples[3, i])) q^(i)
```

---

### W3

- com[, ] defines the commutator.

```
In[13]:= com[L[n_], L[m_]] := If[n + m == 0, c (n^3 - n) / 12 Id[], 0] + (n - m) L[n + m]
In[14]:= com[L[n_], W[m_]] := (2 n - m) W[n + m]
In[15]:= com[W[m_], L[n_]] := -(2 n - m) W[n + m]
```

- The definition of W[n] is  $\text{Sqrt}[(5c+22)/216]$  times the “normal” one. This definition is more natural from the point of view of the Miura transform

```
In[16]:= com[W[n_], W[m_]] :=
  (1 / 48) ( (22 + 5 c) c / (3 * 5!) (n^2 - 1) (n^2 - 4) n If[n + m == 0, 1, 0] Id[] + 16 (n - m)  $\Lambda$ [n + m] +
  (22 + 5 c) (n - m) ((n + m + 2) (n + m + 3) / 15 - (n + 2) (m + 2) / 6) L[n + m] )
In[17]:=  $\Lambda$ [n_] := Module[{m}, Sum[L[m] ** L[n - m], {m, -10, -2}] + Sum[L[n - m] ** L[m], {m, -1, 10}]] -
  (3 / 10) (n + 2) (n + 3) L[n]
```

- Helper functions for the normal ordering. First, we classify operators into Cartans, annihilators and creators

```
In[18]:= cartanQ[J_[n_]] := n == 0
```

```
In[19]:= annQ[J_[n_]] := n > 0
```

```
In[20]:= creQ[J_[n_]] := n < 0
```

■ Assign lexicographic values to operators. We'll reorder the operators accodring this o[ ... ].

```
In[21]:= o[L[n_]] := 1000 n
```

```
In[22]:= o[W[n_]] := n
```

```
In[23]:= o[ket[]] := 1 000 000 000
```

```
In[24]:= o[bra[]] := -1 000 000 000
```

■ Eigenvalue of the Cartan elements.

```
In[25]:= value[L[0]] := Δ
```

```
In[26]:= value[W[0]] := w
```

■ Here follows the main reordering logic. It's a straightforward implementation of what we do on paper.

```
In[27]:= algQ[x_] := MatchQ[x, Id[] | W[_] | L[_]]
```

```
In[28]:= Q[a___, Id[], b___] := Q[a, b]
```

```
In[29]:= Q[x___, a_, ket[]] /; annQ[a] := 0
```

```
In[30]:= Q[x___, a_, ket[]] /; cartanQ[a] := value[a] Q[x, ket[]]
```

```
In[31]:= Q[bra[], a_, x___] /; creQ[a] := 0
```

```
In[32]:= Q[bra[], a_, x___] /; cartanQ[a] := value[a] Q[bra[], x]
```

```
In[33]:= Q[bra[], ket[]] := 1
```

```
In[34]:= Q[x___, a_, b_, y___] /; o[a] > o[b] := Q[x] ** com[a, b] ** Q[y] + Q[x, b, a, y]
```

```
In[35]:= Unprotect[NonCommutativeMultiply];
```

```
In[36]:= NonCommutativeMultiply /: op_ ** Q[x___] /; algQ[op] := Q[op, x]
```

```
In[37]:= NonCommutativeMultiply /: Q[x___] ** op_ /; algQ[op] := Q[x, op]
```

```
In[38]:= NonCommutativeMultiply /: (a_ + b_) ** c_ := a ** c + b ** c
```

```
In[39]:= NonCommutativeMultiply /: a_ ** (b_ + c_) := a ** b + a ** c
```

```
In[40]:= NonCommutativeMultiply /: a_ ** (b_ Q[x___]) := b (a ** Q[x])
```

```
In[41]:= NonCommutativeMultiply /: (b_ Q[x___]) ** a_ := b (Q[x] ** a)
```

```
In[42]:= NonCommutativeMultiply /: (a_ b_) ** c_ /; FreeQ[a, Q] := a (b ** c)
```

```
In[43]:= NonCommutativeMultiply /: a_ ** (b_ c_) /; FreeQ[b, Q] := b (a ** c)
```

```
In[44]:= NonCommutativeMultiply /: Q[x___] ** Q[y___] := Q[x, y]
```

```
In[45]:= NonCommutativeMultiply /: a_ ** 0 := 0
```

```
In[46]:= NonCommutativeMultiply /: 0 ** a_ := 0
```

```
In[47]:= NonCommutativeMultiply /: a_ ** Id[] /; algQ[a] := a
```

```
In[48]:= NonCommutativeMultiply /: Id[] ** a_ /; algQ[a] := a
```

```
In[49]:= Protect[NonCommutativeMultiply];
```

■ Now we define basis vectors of the Verma module and its dual.

```
In[50]:= bra[{Y1_, Y2_}] := Q @@ (Join[{bra[]}, W/@ Reverse[Y2], L/@ Reverse[Y1]])
```

```
In[51]:= ket[{Y1_, Y2_}] := Q @@ (Join[L /@ -Y1, W /@ -Y2, {ket[]}])
```

■ Shapovalov matrix.

```
In[52]:= Shap[n_] := Shap[n] = Module[{x = YoungTuples[2, n], i, j},
  Table[(bra[x[[i]]] ** ket[x[[j]])] // Expand, {i, 1, Length[x]}, {j, 1, Length[x]}]]
```

■ The vector  $W_{-1} W_{-1} \dots W_{-1} | \Delta, w \rangle$  happen to live at this position in our convention.

```
In[53]:= pos[n_] := pos[n] = (*Position[YoungTuples[2, n], {{}, Table[1, {i, 1, n}]]][[1]][[1]]*)
  Length[IntegerPartitions[n]]
```

■ So this is the contribution from grade  $n$ , in the naive implementation.

```
In[54]:= ww[n_] := Inverse[Shap[n]] [[pos[n], pos[n]]]
```

■ But this is slightly faster.

```
In[55]:= vec[n_] := Module[{x = Length[YoungTuples[2, n]], i}, Table[If[i == pos[n], 1, 0], {i, 1, x}]]
```

```
In[56]:= ww[n_] := LinearSolve[Shap[n], vec[n]] [[pos[n]]] λλ^n
```

■ But it's impossible to carry out in general; here we can substitute numerical values before taking the inverse.

```
In[57]:= ww[n_, rep_] := LinearSolve[Shap[n] /. dic /. rep, vec[n]] [[pos[n]]]
```

## Comparison

■ Dictionary. We fix the rescaling of  $\epsilon_{1,2}$  and  $a_{1,2}$  by demanding  $\epsilon_1 \epsilon_2 = 1$

```
In[58]:= e1 = b; e2 = 1 / b;
```

```
In[59]:= dic := {c → 2 + 24 (b + 1 / b) ^ 2, Δ → -a1 ^ 2 - a1 a2 - a2 ^ 2 + (b + 1 / b) ^ 2, w → I a1 a2 (a1 + a2), λλ → q}
```

```
In[60]:= k = 1;
```

```
In[61]:= Shap[k] // Simplify // MatrixForm
```

```
Out[61]//MatrixForm=
```

$$\begin{pmatrix} \frac{1}{48} \Delta (2 - c + 32 \Delta) & 3 w \\ 3 w & 2 \Delta \end{pmatrix}$$

```
In[62]:= cft = ww[k]
```

```
Out[62]=
```

$$\frac{48 \Delta \lambda \lambda}{-216 w^2 + 2 \Delta^2 - c \Delta^2 + 32 \Delta^3}$$

```
In[63]:= gauge = pure[k]
```

```
Out[63]=
```

$$q \left( \frac{1}{(-2 a_1 - a_2) \left( \frac{1}{b} + b + a_1 - a_2 \right) (-a_1 + a_2) \left( \frac{1}{b} + b + 2 a_1 + a_2 \right)} + \frac{1}{\left( \frac{1}{b} + b - a_1 - 2 a_2 \right) \left( \frac{1}{b} + b - 2 a_1 - a_2 \right) (2 a_1 + a_2) (a_1 + 2 a_2)} + \frac{1}{(-a_1 - 2 a_2) (a_1 - a_2) \left( \frac{1}{b} + b - a_1 + a_2 \right) \left( \frac{1}{b} + b + a_1 + 2 a_2 \right)} \right)$$

```
In[64]:= gauge - cft /. dic // FullSimplify
```

```
Out[64]= 0
```

```
In[65]:= k = 2;
```

```
In[66]:= Shap[k] // Simplify // MatrixForm
```

```
Out[66]//MatrixForm=
```

$$\begin{pmatrix} \frac{1}{6} \Delta (6 + c + 8 \Delta) & \frac{1}{8} w (14 + c + 48 \Delta) & \frac{1}{12} \Delta (2 - c + 32 \Delta) \\ \frac{1}{8} w (14 + c + 48 \Delta) & \frac{27648 w^2 + \Delta (c^2 (1+2 \Delta) - 4 c (9+26 \Delta+32 \Delta^2) + 4 (17+306 \Delta+576 \Delta^2+512 \Delta^3))}{2304} & -\frac{1}{16} w (-2 + c - 32 \Delta) (3 + 2 \Delta) \\ \frac{1}{12} \Delta (2 - c + 32 \Delta) & -\frac{1}{16} w (-2 + c - 32 \Delta) (3 + 2 \Delta) & \frac{1}{24} (216 w^2 - (-2 + c - 32 \Delta) \Delta (1 \\ 6 w & -\frac{5}{48} (-2 + c - 32 \Delta) \Delta & 9 w \\ 12 w & 18 w^2 + \frac{1}{8} \Delta (2 - c + 32 \Delta) & 6 (w + 2 w \Delta) \end{pmatrix}$$

```
In[67]:= cft = ww[k]
```

```
In[68]:= gauge = pure[k]
```

```
In[69]:= gauge - cft /. dic // FullSimplify
```

```
Out[69]= 0
```

```
In[70]:= repl = {a1 -> Random[Integer, 200],  
                a2 -> Random[Integer, 200], b -> Random[Integer, 200], q -> 1}
```

```
Out[70]= {a1 -> 173, a2 -> 35, b -> 86, q -> 1}
```

```
In[71]:= k = 3;
```

```
In[72]:= Shap[k] // Simplify // MatrixForm
```

```
In[73]:= cft = ww[k, repl]
```

```
Out[73]= 6 774 707 040 914 741 792 194 413 371 550 734 255 861 502 259 395 639 916 243 226 718 043 394 556 842 768 \
          939 836 672 /
          4 037 310 376 217 635 098 953 963 217 501 895 681 883 892 670 202 679 927 832 068 968 585 706 176 646 441 \
          493 866 074 374 835 606 249 802 127 651 715 625
```

```
In[74]:= gauge = pure[3] /. repl
```

```
Out[74]= 6 774 707 040 914 741 792 194 413 371 550 734 255 861 502 259 395 639 916 243 226 718 043 394 556 842 768 \
          939 836 672 /
          4 037 310 376 217 635 098 953 963 217 501 895 681 883 892 670 202 679 927 832 068 968 585 706 176 646 441 \
          493 866 074 374 835 606 249 802 127 651 715 625
```

```
In[75]:= cft - gauge
```

```
Out[75]= 0
```
